# Supplementary material for: Spatiotemporal k-means
Source: arXiv:2211.05337 source file (2024-04-15)
Supplement: Supplementary file 1 [file 10_appendix_init.tex]

\appendix
\section{Supplementary Material}
\subsection{Code}
Code can be found at:
\\
\url{https://github.com/OlgaD400/STKM}
